# Supplementary material for: Publicly Auditable MPC-as-a-Service with succinct verification and universal setup
Source: arXiv:2107.04248 source file (2021-07-09)
Supplement: Supplementary file 1 [file comm_cost_details.tex]

\section{Detailed breakdown of communication cost:}
\label{app:comm_breakdown}

Table \ref{table:round_analysis} shows the detailed round wise communication cost analysis for each round(these rounds are different from the marlin rounds) when clients commit with \textsf{PEC.Poly}. In the initial round, the servers exchange the commitments to shares of statements and validate that clients inputs are consistent with the commitments on the bulletin board. 
In the first round, the servers commit to the secret shared polynomials $w, x, mask, z_a, z_b$. The second round of communication consists of 2 commitments to secret shared polynomials $g_1, h_1$. The polynomial $g_1$ has a strict degree bound and hence the it is equivalent to two commitments(See Appendix D of Marlin~\cite{chiesa2019marlin}). In the third round, the evaluations for $g_1, h_1, x, w, mask, z_a, z_b$ at $\beta_1$ are opened and finally in the last round, a batch proof over these evaluations is created. 

\begin{table}[ht!]
 \caption{Communication Cost in terms of number of openings. $N$ represents the number of MPC servers and $|X|$ is the statement size. \label{table:round_analysis}}
\resizebox{\columnwidth}{!}{%
 \begin{tabular}{||c| c| c c c||} 
 \hline
 - & Msg Type & $\mathbb{G}_1$ & $\mathbb{G}_2$ & $\mathbb{F}_q$ \\ [0.5ex] 
 \hline\hline
 Initial Round & commitments & $|X| + 1$ & - & - \\ 
 \hline
 First Round & commitments & $4$ & - & - \\
 \hline
 Second Round & commitments & $3$ & - & - \\
 \hline
 Third Round & evaluations & - & - & $7$ \\
 \hline
  Fourth Round & PolyEval proofs & $1$ & - & $1$ \\
 \hline
%  \multirow{3}{1cm}{Second Round} & commitments &$2$ & - & - \\
%                                 & PolyEval proofs &$6$ & - & $6$ \\
%                                 & evaluations & - & - & $8$ \\
%  \hline
\end{tabular}
}
 \end{table}
